# Supplementary material for: General H-theorem and entropies that violate the second law
Source: arXiv:1212.6767 ancillary file (2014-10-09)
Supplement: Supplementary file 1 [file NewEntropy2014.pdf]

# New universal Lyapunov functions for nonlinear kinetics

Alexander N. Gorban

Department of Mathematics  
University of Leicester, UK

July 21, 2014, Leicester

# Outline

- 1 Relative entropy and divergences
  - Classical relative entropy and  $H$ -theorems
  - $f$ -divergences and Rényi–Csiszár–Morimoto  $H$ -theorems
  - The most popular examples of  $H_h(P\|P^*)$
- 2 Maximum of quasiequilibrium relative entropies
  - Quasiequilibrium relative entropy
  - New Lyapunov functions
  - Forward–invariant peeling

# Outline

## 1 Relative entropy and divergences

- Classical relative entropy and  $H$ -theorems
- $f$ -divergences and Rényi–Csiszár–Morimoto  $H$ -theorems
- The most popular examples of  $H_h(P\|P^*)$

## 2 Maximum of quasiequilibrium relative entropies

- Quasiequilibrium relative entropy
- New Lyapunov functions
- Forward–invariant peeling

# Boltzmann–Gibbs–Shannon relative entropy (1872–1948)

For a system with discrete space of states  $A_i$

$$H_{\text{BGS}}(P\|P^*) = \sum_i p_i \left( \ln \left( \frac{p_i}{p_i^*} \right) - 1 \right)$$

where  $P = (p_i)$ ,  $P^* = (p_i^*)$  are the positive probability distributions.

# Kolmogorov's (master) equation

$$q_{ij} = q_{i \leftarrow j} \geq 0 \text{ for } i \neq j \ (i, j = 1, \dots, n)$$

$$\frac{dp_i}{dt} = \sum_{j, j \neq i} (q_{ij} p_j - q_{ji} p_i)$$

With a known positive equilibrium  $P^*$

$$\frac{dp_i}{dt} = \sum_{j, j \neq i} q_{ij} p_j^* \left( \frac{p_j}{p_j^*} - \frac{p_i}{p_i^*} \right)$$

where  $p_i^*$  and  $q_{ij}$  are connected by the *balance equation*

$$\sum_{j, j \neq i} q_{ij} p_j^* = \left( \sum_{j, j \neq i} q_{ji} \right) p_i^* \text{ for all } i = 1, \dots, n$$

# Information processing lemma (continuous time)

Information does not increase (in average) due to random manipulations (Shannon 1948).

For a system with positive equilibrium  $P^*$

$$\frac{d}{dt} H_{\text{BGS}}(P\|P^*) \leq 0$$

due to master equation

# Mass action law

- $A_i$  are components,  $c_i$  is concentration of  $A_i$
- $\sum_i \alpha_{ri} A_i \rightleftharpoons \sum_i \beta_{ri} A_i$  – elementary reactions (reversible)
- $w_r^+ = k_r^+ \prod_i c_i^{\alpha_{ri}}$ ,  $w_r^- = k_r^- \prod_i c_i^{\beta_{ri}}$ ;
- $w_r = w_r^+ - w_r^-$  – the reaction rate
- $\gamma_r = (\gamma_{ri}) = (\beta_{ri} - \alpha_{ri})$  – the stoichiometric vector
- $\dot{c} = \sum_r \gamma_r w_r$  – kinetic equations

# Detailed balance and $H$ -theorem (essentially, Boltzmann, 1872)

There exists a positive point of detailed balance:

$$c_i^* > 0, \forall r \quad w_r^+(c^*) = w_r^-(c^*)$$

Then for all positive  $c$

$$\begin{aligned} \frac{d}{dt} \sum_i c_i \left( \ln \left( \frac{c_i}{c_i^*} \right) - 1 \right) \\ = - \sum_r (w_r^+ - w_r^-) (\ln w_r^+ - \ln w_r^-) \leq 0 \end{aligned}$$



# Outline

- 1 Relative entropy and divergences
  - Classical relative entropy and  $H$ -theorems
  - $f$ -divergences and Rényi–Csiszár–Morimoto  $H$ -theorems
  - The most popular examples of  $H_h(P\|P^*)$
- 2 Maximum of quasiequilibrium relative entropies
  - Quasiequilibrium relative entropy
  - New Lyapunov functions
  - Forward–invariant peeling

# $f$ -divergences

For any convex function  $h(x)$  defined on the open ( $x > 0$ ) or closed  $x \geq 0$  semi-axis

$$H_h(p) = H_h(P\|P^*) = \sum_i p_i^* h\left(\frac{p_i}{p_i^*}\right)$$

where  $P = (p_i)$  is a probability distribution,  $P^*$  is an equilibrium distribution.

Rényi (1960) Csiszár (1963), and Morimoto (1963) proved the information processing lemma ( $H$ -theorem) for these functions and Markov chains.

# Rényi–Csiszár–Morimoto $H$ -theorem

Due to Master equation with the positive equilibrium  $P^*$

$$\begin{aligned}\frac{dH_h(p)}{dt} &= \sum_{i,j,i \neq j} h' \left( \frac{p_j}{p_j^*} \right) q_{ji} p_i^* \left( \frac{p_i}{p_i^*} - \frac{p_j}{p_j^*} \right) \\ &= \sum_{i,j,i \neq j} q_{ij} p_j^* \left[ h \left( \frac{p_i}{p_i^*} \right) - h \left( \frac{p_j}{p_j^*} \right) + h' \left( \frac{p_i}{p_i^*} \right) \left( \frac{p_j}{p_j^*} - \frac{p_i}{p_i^*} \right) \right] \leq 0\end{aligned}$$

# Outline

## 1 Relative entropy and divergences

- Classical relative entropy and  $H$ -theorems
- $f$ -divergences and Rényi–Csiszár–Morimoto  $H$ -theorems
- The most popular examples of  $H_h(P\|P^*)$

## 2 Maximum of quasiequilibrium relative entropies

- Quasiequilibrium relative entropy
- New Lyapunov functions
- Forward–invariant peeling

# Hartley & BGS

- $h(x)$  is the step function,  $h(x) = 0$  if  $x = 0$  and  $h(x) = -1$  if  $x > 0$ .

$$H_h(P\|P^*) = - \sum_{i, p_i > 0} 1.$$

(the Hartley entropy);

- $h = |x - 1|$ ,

$$H_h(P\|P^*) = \sum_i |p_i - p_i^*|;$$

(the  $l_1$ -distance between  $P$  and  $P^*$ );

- $h = x \ln x$ ,

$$H_h(P\|P^*) = \sum_i p_i \ln \left( \frac{p_i}{p_i^*} \right) = D_{\text{KL}}(P\|P^*);$$

(the relative Boltzmann–Gibbs–Shannon (BGS) entropy);

# Burg & Fisher

- $h = -\ln x$ ,

$$H_h(P\|P^*) = -\sum_i p_i^* \ln\left(\frac{p_i}{p_i^*}\right) = H_{\text{BGS}}(P^*\|P);$$

(the relative Burg entropy);

- $h = \frac{(x-1)^2}{2}$ ,

$$H_h(P\|P^*) = \frac{1}{2} \sum_i \frac{(p_i - p_i^*)^2}{p_i^*} = H_2(P\|P^*);$$

(the quadratic approximation of the relative  
Boltzmann–Gibbs–Shannon entropy);

# Cressie–Read (CR) family

- $h = \frac{x(x^\lambda - 1)}{\lambda(\lambda + 1)}$

$$H_h(P\|P^*) = \frac{1}{\lambda(\lambda + 1)} \sum_i p_i \left[ \left( \frac{p_i}{p_i^*} \right)^\lambda - 1 \right];$$

(the Cressie–Read (CR) family).

If  $\lambda \rightarrow 0$  then  $H_{\text{CR } \lambda} \rightarrow H_{\text{BGS}}$ ,

if  $\lambda \rightarrow -1$  then  $H_{\text{CR } \lambda} \rightarrow H_{\text{Burg}}$ ;

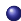

$$H_{\text{CR } \infty}(P\|P^*) = \max_i \left\{ \frac{p_i}{p_i^*} \right\} - 1;$$

$$H_{\text{CR } -\infty}(P\|P^*) = \max_i \left\{ \frac{p_i^*}{p_i} \right\} - 1.$$

# Tsallis

- $h = \frac{(x^\alpha - x)}{\alpha - 1}, \alpha > 0,$

$$H_h(P\|P^*) = \frac{1}{\alpha - 1} \sum_i p_i \left[ \left( \frac{p_i}{p_i^*} \right)^{\alpha - 1} - 1 \right].$$

(the Tsallis relative entropy).



# The puzzle of nonlinear systems

- For the linear systems many Lyapunov functionals are known in the explicit form,
- On the contrary, for the nonlinear MAL systems with detailed balance we, typically, know the only Lyapunov function  $H_{\text{BGS}}$ ;
- The situation looks rather intriguing and challenging: for every finite reaction mechanism with detailed balance there **should be** many Lyapunov functionals, but we cannot construct them.
- We present a general procedure for the construction of a family of new Lyapunov functionals from  $H_{\text{BGS}}$  for nonlinear MAL kinetics and a given reaction mechanism.
- There is no chance to find many Lyapunov functions for *all* nonlinear mechanisms together.

# Outline

- 1 Relative entropy and divergences
  - Classical relative entropy and  $H$ -theorems
  - $f$ -divergences and Rényi–Csiszár–Morimoto  $H$ -theorems
  - The most popular examples of  $H_h(P\|P^*)$
- 2 Maximum of quasiequilibrium relative entropies
  - Quasiequilibrium relative entropy
  - New Lyapunov functions
  - Forward-invariant peeling

# Quasiequilibrium

Let

$$H(c) = H_{\text{BGS}}(c) = \sum_i c_i \left( \ln \left( \frac{c_i}{c_i^*} \right) - 1 \right)$$

For every linear subspace  $E \subset \mathbb{R}^n$  and a given concentration vector  $c^0 \in \mathbb{R}_+^n$  the *quasiequilibrium composition* is the conditional minimizer of  $H$ :

$$c_E^*(c^0) = \operatorname{argmin}_{c \in (c^0 + E) \cap \mathbb{R}_+^n} H(c)$$

The *quasiequilibrium divergence* is the value of  $H$  at the quasiequilibrium:

$$H_E^*(c^0) = \min_{c \in (c^0 + E) \cap \mathbb{R}_+^n} H(c)$$

# Properties of quasiequilibria

- $H$  is strongly convex and  $\nabla H$  has logarithmic singularity at  $c_i \rightarrow 0$ .
- Therefore, for a positive vector  $c^0 \in \mathbb{R}_+^n$  and a given subspace  $E \subset \mathbb{R}^n$  the quasiequilibrium composition  $c_E^*(c^0)$  is also positive.

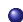

$$H_E^*(c^0) \leq H(c^0)$$

and this inequality turns into the equality if and only if  $c^0$  is the quasiequilibrium  $c^0 = c_E^*(c^0)$ .

- Such quasiequilibrium “entropies” were discussed by Jaynes (1965).
- He considered the quasiequilibrium  $H$ -function as the Boltzmann  $H$ -function  $H_B$  in contrast to the original Gibbs  $H$ -function,  $H_G$ .
- The Gibbs  $H$ -function is defined for the distributions on the phase space of the mechanical systems. The Boltzmann function is a conditional minimum of the Gibbs function, therefore the Jaynes inequality holds

$$H_B \leq H_G$$

- These functions are intensively used in the discussion of time arrow.
- In the theory of information, quasiequilibrium was studied in detail under the name *information projection*.

- Consider the reversible reaction mechanism with the set of the stoichiometric vectors  $\Upsilon$ .
- For each  $\Gamma \subset \Upsilon$  we can take  $E = \text{Span}(\Gamma)$  and define the quasiequilibrium.
- Let  $\mathcal{E}_\Upsilon$  be the set of all subspaces of the form  $E = \text{Span}(\Gamma)$  ( $\Gamma \subset \Upsilon$ ).
- $\mathcal{E}_\Upsilon^k$  is the set of  $k$ -dimensional subspaces from  $\mathcal{E}_\Upsilon$  for each  $k$ .
- Define  $H_\Upsilon^{k,\max}$  for each dimension  $k = 0, \dots, \text{rank}(\Upsilon)$ :  
 $H_\Upsilon^{0,\max} = H$ , and for  $k > 0$

$$H_\Upsilon^{k,\max}(c) = \max_{E \in \mathcal{E}_\Upsilon^k} H_E^*(c)$$

# Outline

- 1 Relative entropy and divergences
  - Classical relative entropy and  $H$ -theorems
  - $f$ -divergences and Rényi–Csiszár–Morimoto  $H$ -theorems
  - The most popular examples of  $H_h(P\|P^*)$
- 2 Maximum of quasiequilibrium relative entropies
  - Quasiequilibrium relative entropy
  - **New Lyapunov functions**
  - Forward-invariant peeling

$H^{1,\max}$ 

$$H_{\Upsilon}^{1,\max}(c^0) = \max_{\gamma \in \Upsilon} \left\{ \min_{c \in (c^0 + \gamma \mathbb{R}) \cap \mathbb{R}_+^n} H(c) \right\}$$

$H_{\Upsilon}^{1,\max}(c)$  is a Lyapunov function in  $\mathbb{R}_+^n$  for all MAL systems with the given equilibrium  $c^*$  and detailed balance on the set of stoichiometric vectors  $\Gamma \subseteq \Upsilon$ .



# Simple reaction mechanism for example

Consider a simple reaction mechanism:

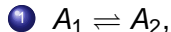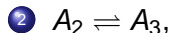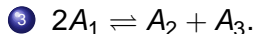

The concentration triangle  $c_1 + c_2 + c_3 = b$  is split by the partial equilibria lines into six compartments.

# Example: QE states

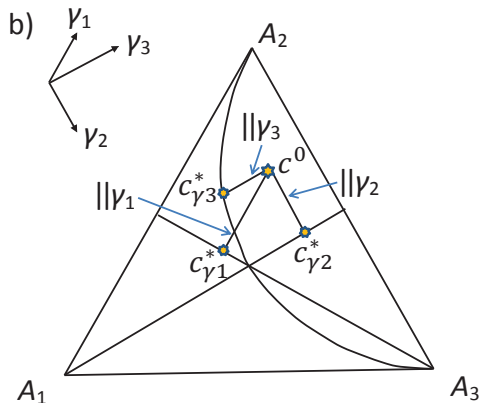

## Example: $H^{1,\max}$ level set

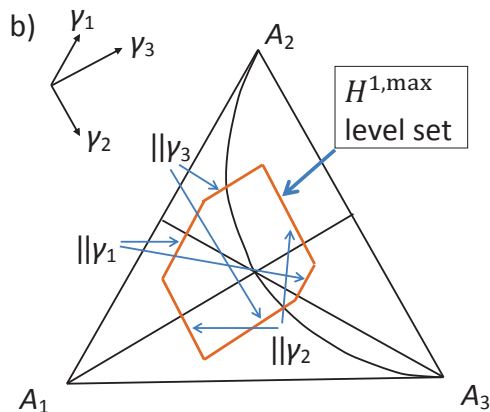

# Outline

- 1 Relative entropy and divergences
  - Classical relative entropy and  $H$ -theorems
  - $f$ -divergences and Rényi–Csiszár–Morimoto  $H$ -theorems
  - The most popular examples of  $H_h(P\|P^*)$
- 2 Maximum of quasiequilibrium relative entropies
  - Quasiequilibrium relative entropy
  - New Lyapunov functions
  - Forward-invariant peeling

- Let  $U$  be a convex compact set of non-negative  $n$ -dimensional vectors  $c$  and for some  $\eta > \min H$  the  $\eta$ -sublevel set of  $H$  belongs to  $U$ :  $\{N \mid H(N) \leq \eta\} \subset U$ .
- Let  $h > \min H$  be the maximal value of such  $\eta$ .
- Select  $\varepsilon > 0$ . The  $\varepsilon > 0$ -peeled set  $U$  is

$$U_{\Upsilon}^{\varepsilon} = U \cap \{N \in \overline{R_+^n} \mid H_{\Upsilon}^{1, \max}(N) \leq h - \varepsilon\}$$

- For sufficiently small  $\varepsilon > 0$  ( $\varepsilon < h - \min H$ ) this set is non-empty and forward-invariant.

# Illustration: forward-invariant peeling

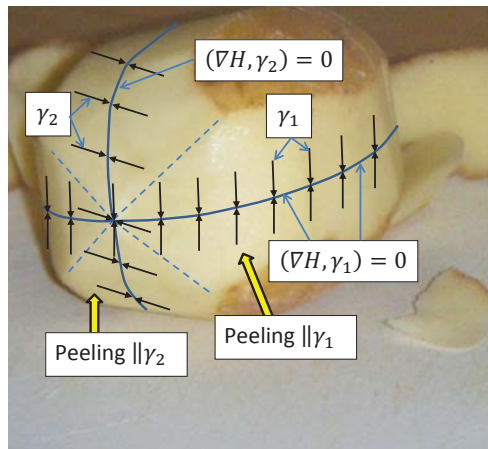

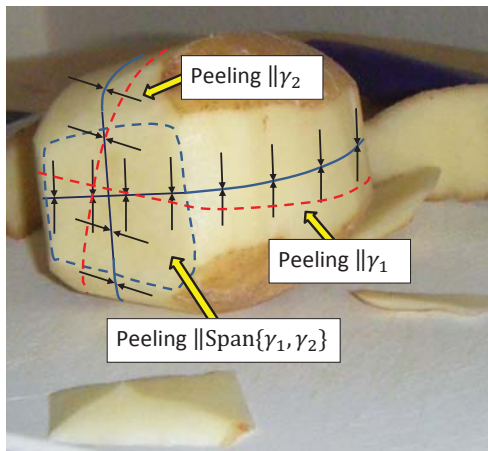

The additional peeling  $\|\text{Span}\{\gamma_1, \gamma_2\}$  makes the peeled set forward-invariant with respect to the set of systems with interval reaction rate constants.

# Main message

- For every reaction mechanism there exists an infinite family of Lyapunov functions for reaction kinetics that depend on the equilibrium but not in the rate constants.
- These functions are produced by the operations of conditional minimization and maximization from the BGS relative entropy.



# References

A.N. Gorban, General H-theorem and entropies that violate the second law, *Entropy* 2014, 16(5), 2408-2432. **Extended postprint arXiv:1212.6767** [cond-mat.stat-mech], <http://arxiv.org/pdf/1212.6767.pdf> (43 pages).  
Just look Gorban in arXiv and references there.
